# Supplementary material for: Unraveling the Atomic-Scale Pathways Driving Pressure-Induced Phase Transitions in Silicon
Source: arXiv:2408.12358 source file (2024-08-22)
Supplement: Supplementary file 1 [file Supplementary_Material_Transitions.pdf]

# Supplementary Material: Unraveling the Atomic-Scale Pathways Driving Pressure-Induced Phase Transitions in Silicon

Fabrizio Rovaris *[1], Anna Marzegalli[1], Francesco Montalenti[1], and Emilio Scalise[1]

[1] *Department of Materials Science. University of Milano Bicocca, Via R. Cozzi 55, I-20125, Milano, Italy*

## S1 Additional tests for the GAP potential

In this Section we report some additional details regarding the comparison we performed for testing the accuracy of the GAP potential with respect to DFT calculations regarding kinetic barrier estimation.

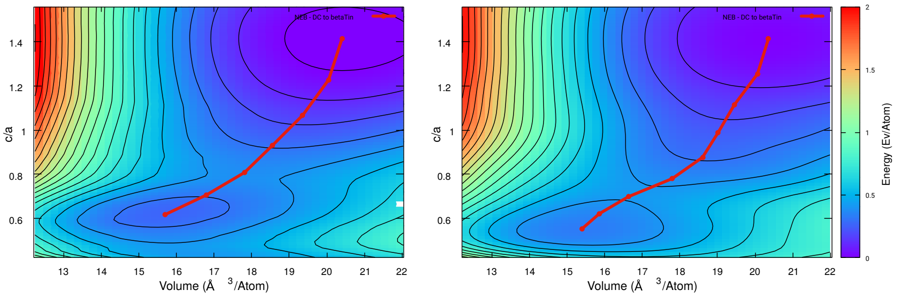


Figure S1: Potential Energy Surface for the meighborhood of the *dc* and $\beta$-Sn phases as evaluated by DFT (a) and the GAP potential (b). The Minimum Energy Path found by SS-NEB calculations is reported as a red line on each plot.

As a first comparison we investigated the atomic neighborhood of the *dc* and $\beta$-Sn phases in the Potential Energy Surface (PES). Since these two phases have very close

*Corresponding author: fabrizio.rovaris@unimib.it

crystallographic structures their PES neighborhood can be described by just two global variables: the Volume per atom and the c/a ratio of their crystallographic cells. Indeed, one phase can be transformed into the other by just affine transformation of the cells, while keeping the atom fixed in their (transformed) positions. We thus explored the PES by repeating DFT and GAP calculations starting from the *dc* phase and deforming the cell in the c/a ration and the volume. We reported our results as color-plots in Fig. S1(a) and (b) for, respectively, DFT and GAP calculations. As can be appreciated in the figure the agreement is excellent, confirming the accuracy of the GAP potential also in regions far away from the equilibrium configuration of the phases.

Moreover, as mentioned in the main text, we repeated SS-NEB calculations in order to find the Minimum Energy Path connecting the two phases for both GAP and DFT. The resulting transition paths are plotted as red lines in Fig. S1. Again, the agreement is excellent and it is also confirmed by the energy barrier comparison reported in Fig. 1 of the main manuscript.

# S2 Transition paths

## S2.1 dc to $\beta$-Sn

In figure S2 we report the images taken along the transition path of the *dc* to $\beta$-Sn transition shown in Fig. 2(a) of main manuscript. Snapshots are shown for the top and the side views, in Fig. S2(a) and (b), respectively.

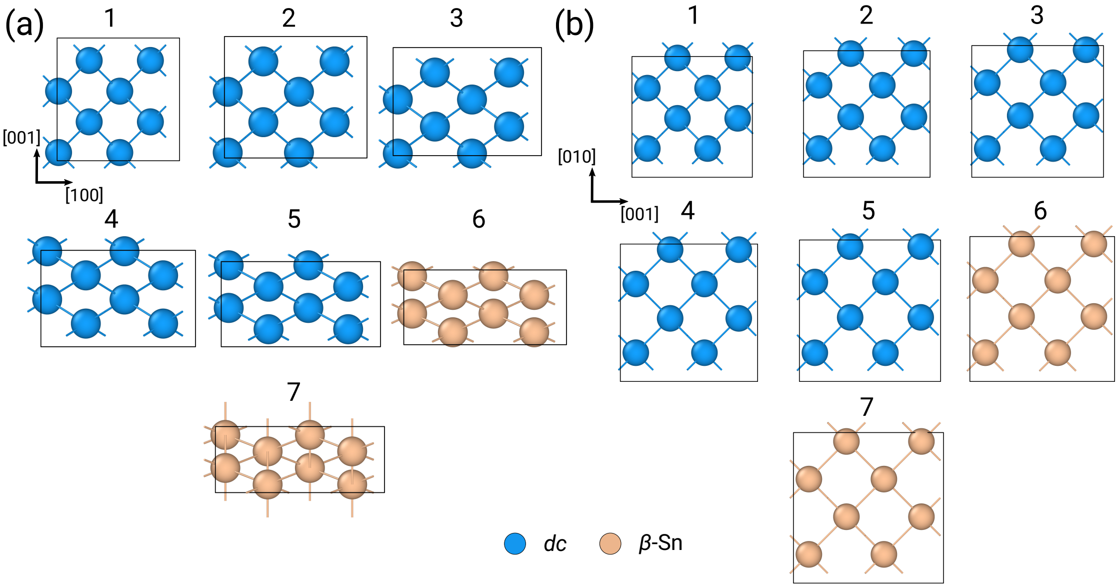


Figure S2: Snapshots taken along the transition path from BC8 to R8, shown in figure 3(b) of the main manuscript. Images are shown from the side and the top views in panels (a) and (b), respectively.

## S2.2 $\beta$-Sn to BC8

In figure S3 we report the images taken along the transition path of the $\beta$-Sn to BC8 transition shown in Fig. 3(a) of main manuscript. Snapshots are shown for the top and the side views, in Fig. S3(a) and (b), respectively.

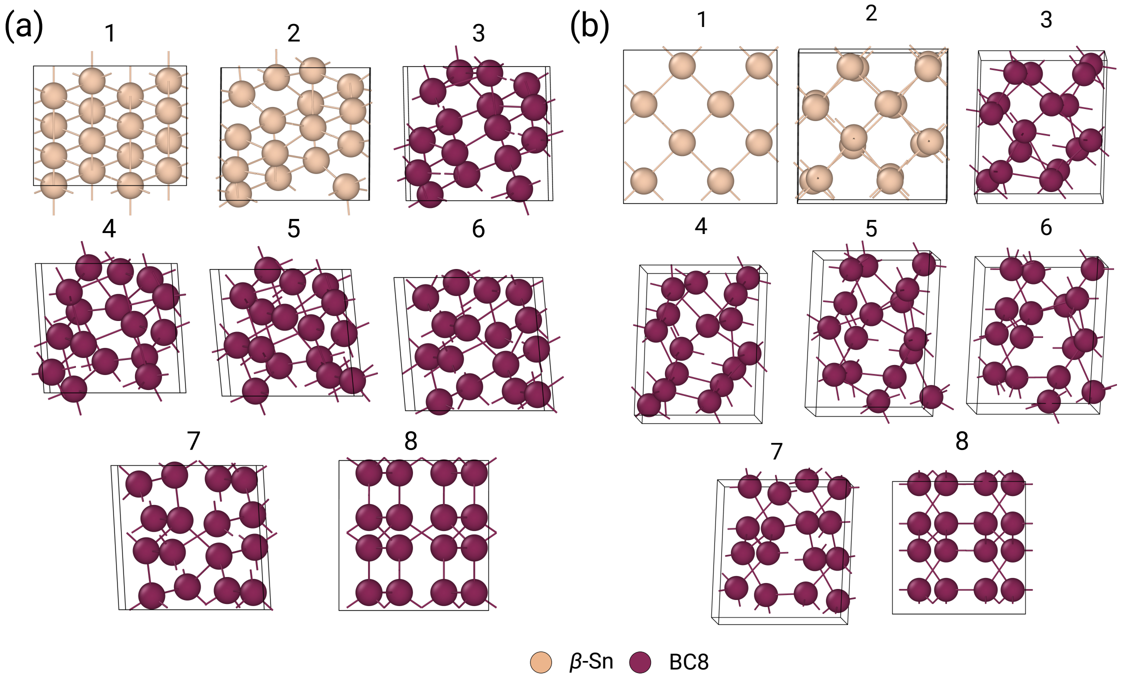


Figure S3: Snapshots taken along the transition path from $\beta$-Sn to BC8, shown in figure 3(a) of the main manuscript. Images are shown from the side and the top views in panels (a) and (b), respectively.

## S2.3 $\beta$-Sn to R8

In figure S4 we report the images taken along the transition path of the $\beta$-Sn to R8 transition shown in Fig. 3(a) of main manuscript. Snapshots are shown for the top and the side views, in Fig. S4(a) and (b), respectively.

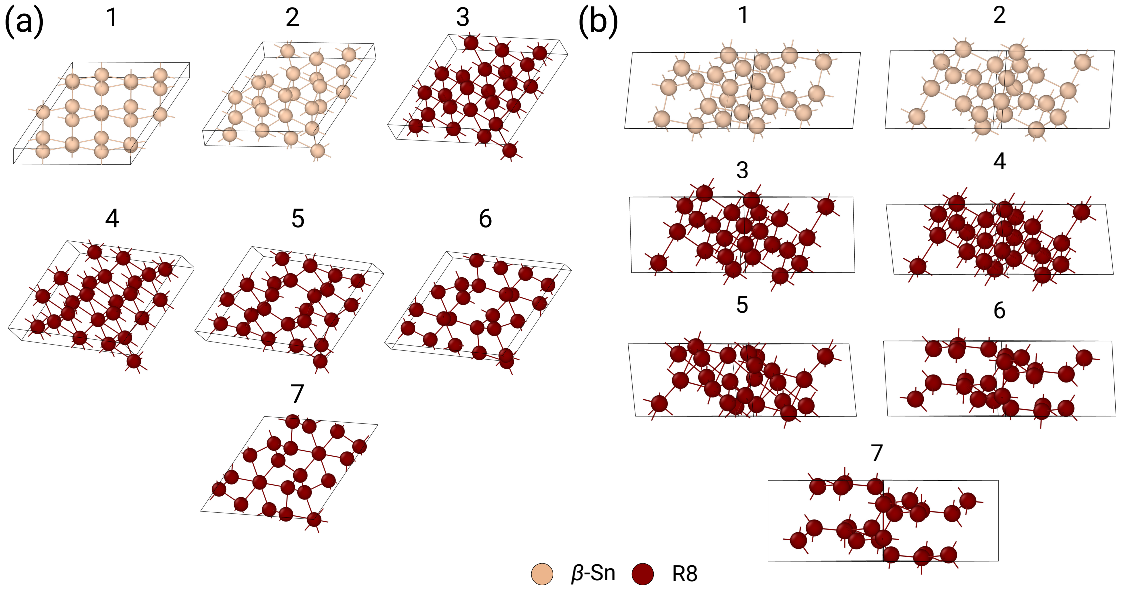


Figure S4: Snapshots taken along the transition path from $\beta$-Sn to R8, shown in figure 3(a) of the main manuscript. Images are shown from the side and the top views in panels (a) and (b), respectively.

## S2.4 BC8 to R8

In figure S5 we report the images taken along the transition path of the BC8 to R8 transition shown in Fig. 3(b) of main manuscript. Snapshots are shown for the top and the side views, in Fig. S5(a) and (b), respectively.

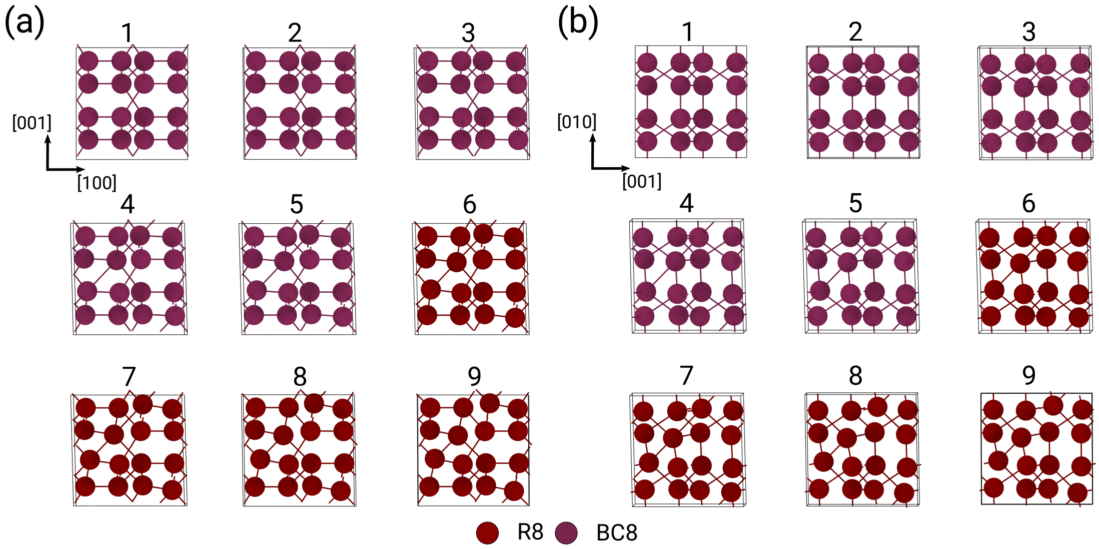


Figure S5: Snapshots taken along the transition path from BC8 to R8, shown in figure 3(b) of the main manuscript. Images are shown from the side and the top views in panels (a) and (b), respectively.

### S2.5 BC8 to hd

In figure S6 we report the images taken along the transition path from BC8 to *hd*, shown in Fig. 4(a) of main manuscript. Snapshots are shown for the top and the side views, in Fig. S6(a) and (b), respectively and crystallographic indexes are reported for the cubic structure.

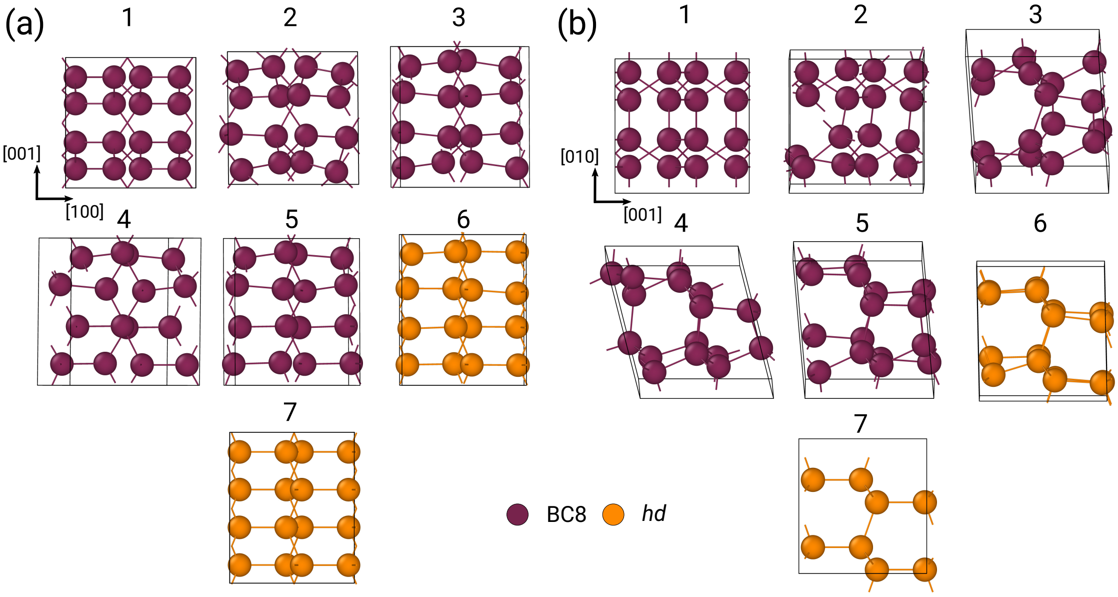


Figure S6: Snapshots taken along the transition path from BC8 to *hd*, shown in figure 4(a) of the main manuscript. Images are shown from the side and the top views in panels (a) and (b), respectively. Crystallographic indexes are reported for the cubic cell
